# Supplementary material for: Transfer Function Models for Cylindrical MC Channels with Diffusion and Laminar Flow
Source: arXiv:2007.01799 source file (2020-07-03)
Supplement: Supplementary file 1 [file appendix.tex]

\textcolor{red}{Uniform flow case}\\
Consider one entry of $\bar{\bm{F}}_\mathrm{uni}(s)$
\begin{align}
\bar{F}_\mathrm{uni}(\mu, s) &= v_0\int_{V}\tilde{K}_3^*(\bm{x},\mu) \bm{c}_1\tran(\bm{x})\dint{\bm{x}} \,\bar{\bm{Y}}(s) \\
&= v_0 \sum_{\tilde{\mu} = 0}^{\infty} \frac{1}{N_{\tilde{\mu}}} 
\int_{V} \tilde{K}_3^*(\bm{x},\mu) K_1(\bm{x},\tilde{\mu})
\dint{\bm{x}}
\bar{Y}(\tilde{\mu},s)\\
&= v_0 \lambda_\nu \sum_{\tilde{\mu} = 0}^\infty\frac{1}{N_{\tilde{\mu}}} 
f_{\mathrm{uni},r}(\mu,\tilde{\mu})\,f_{\mathrm{uni},\varphi}(\mu,\tilde{\mu})\,f_{\mathrm{uni},z}(\mu,\tilde{\mu}) \bar{Y}(\tilde{\mu},s)\\
&= v_0 \lambda_\nu \left[\dots, \, \frac{1}{N_{\tilde{\mu}}} 
f_{\mathrm{uni},r}(\mu,\tilde{\mu})\,f_{\mathrm{uni},\varphi}(\mu,\tilde{\mu})\,f_{\mathrm{uni},z}(\mu,\tilde{\mu}) , \, \dots \right]\bar{\bm{Y}}(s)
\end{align}

\begin{align}
&f_{\mathrm{uni},\varphi}(\mu,\tilde{\mu}) = \int_{-\pi}^{\pi} \expE{\jcomp(n - \tilde{n})}\varphi\dint{\varphi} =  2\pi \delta_{n,\tilde{n}}, 
&\delta_{n,\tilde{n}} = \begin{cases}
1 & n = \tilde{n}\\
0 & n \neq \tilde{n}
\end{cases}
\end{align}
All terms with $n \neq \tilde{n}$ vanish

\begin{align}
f_{\mathrm{uni},r}(\mu,\tilde{\mu}) &= \int_{0}^{R_0} J_n(k_{n,m}r)J_{\tilde{n}}(k_{\tilde{n},\tilde{m}}r)r \dint{r} \\
&\overset{n = \tilde{n}}{=} \int_{0}^{R_0} J_n(k_{n,m}r)J_{n}(k_{n,\tilde{m}}r)r \dint{r} = \frac{R_0^2}{2}
\begin{cases}
0 & m \neq \tilde{m}\\
1 & k_{n,m} = 0, \, n = 0\\
0 & k_{n,m} = 0, \, n \geq 1,\\
\left(1 - \frac{n^2}{k_{n,m}^2}\right)J_n^2(k_{n,m})& k_{n,m} \neq 0, \, m = \tilde{m}\\
\end{cases}
\end{align}
Refer to Arfken Weber \cite[p.~692, Eq.~(11.2.3)]{ArfkenWeber:2001} and therefore it vanishes for $m \neq \tilde{m}$

\begin{align}
f_{\mathrm{uni},z}(\mu,\tilde{\mu}) &= \int_{0}^{Z_0}\cos\lambda_\nu z\sin\lambda_{\tilde{\nu}}z\dint{z} = 
\begin{cases}
0 & \nu = \tilde{nu} = 0\\
0 & \nu \neq 0, \, \tilde{\nu} = 0\\
-\frac{1}{\lambda_{\tilde{\nu}}}\left((-1)^{\tilde{\nu}} - 1 \right) & \nu = 0,\, \tilde{\nu} \neq 0\\
0 & \nu = \tilde{\nu}\\
-\frac{\lambda_{\tilde{\nu}}}{\lambda_{\tilde{\nu}}^2 - \lambda_\nu^2}\left((-1)^{(\tilde{\nu} - \nu)} - 1\right) & \nu \neq \tilde{\nu}
\end{cases}
\end{align}

\textcolor{red}{Parabolic part}\\
Consider one entry of $\bar{\bm{F}}_\mathrm{uni}(s)$
\begin{align}
\bar{F}_\mathrm{lam}(\mu, s) &= - \frac{v_0}{R_0^2}\int_{V}\tilde{K}_3^*(\bm{x},\mu) \bm{c}_1\tran(\bm{x})\dint{\bm{x}} \,\bar{\bm{Y}}(s) \\
&= - \frac{v_0}{R_0^2} \sum_{\tilde{\mu} = 0}^{\infty} \frac{1}{N_{\tilde{\mu}}} 
\int_{V} \tilde{K}_3^*(\bm{x},\mu) K_1(\bm{x},\tilde{\mu})r^2
\dint{\bm{x}}
\bar{Y}(\tilde{\mu},s)\\
&= - \frac{v_0}{R_0^2} \lambda_\nu \sum_{\tilde{\mu} = 0}^\infty\frac{1}{N_{\tilde{\mu}}} 
f_{\mathrm{lam},r}(\mu,\tilde{\mu})\,f_{\mathrm{lam},\varphi}(\mu,\tilde{\mu})\,f_{\mathrm{lam},z}(\mu,\tilde{\mu}) \bar{Y}(\tilde{\mu},s)\\
&= - \frac{v_0}{R_0^2} \lambda_\nu \left[\dots, \, \frac{1}{N_{\tilde{\mu}}} 
f_{\mathrm{lam},r}(\mu,\tilde{\mu})\,f_{\mathrm{lam},\varphi}(\mu,\tilde{\mu})\,f_{\mathrm{lam},z}(\mu,\tilde{\mu}) , \, \dots \right]\bar{\bm{Y}}(s)
\end{align}
Hint that these are lines of the matrix $\Ks_\mathrm{lam}$.

\begin{align}
&f_{\mathrm{uni},\varphi}(\mu,\tilde{\mu}) = f_{\mathrm{lam},\varphi}(\mu,\tilde{\mu}),
&f_{\mathrm{uni},z}(\mu,\tilde{\mu}) = f_{\mathrm{lam},z}(\mu,\tilde{\mu}),
\end{align}
All terms with $n \neq \tilde{n}$ vanish

\begin{align}
f_{\mathrm{lam},r}(\mu,\tilde{\mu}) &= \int_{0}^{R_0} J_n(k_{n,m}r)J_{n}(k_{n,\tilde{m}}r)r^3 \dint{r} 
\end{align}
Can only be solved in closed form for $n = 0$. For $n\neq 0$ integral has to be solved numerically. But only one time!
